# Supplementary material for: Style Variable and Irrelevant Learning for Generalizable Person Re-identification
Source: arXiv:2209.05235 source file (2022-09-12)
Supplement: Supplementary file 1 [file appendix.tex]

% ------------- addendix -----------------------------
% \appendix
